# Supplementary material for: Runtime Backdoor Detection for Federated Learning via Representational Dissimilarity Analysis
Source: arXiv:2503.04473 source file (2025-03-06)
Supplement: Supplementary file 1 [file sec_appendix.tex]

% if have a single appendix:
%\appendix[Proof of the Zonklar Equations]
% or
%\appendix  % for no appendix heading
% do not use \section anymore after \appendix, only \section*
% is possibly needed
\appendix

% \section{Experiment evaluation}
% \subsection{E}

\section{Proofs}
This section provides proof details for Lemma 1-3, Theorem 1 and 2.

\lemmaBenign*
\xz{
\begin{proof}
% Without loss of generality,
Assume any two clients $c_{i_1}$ and $c_{i_2}$ satisfying that $c_{i_1} \in N_{k}(c_{i_2})$, $c_{i_2} \in N_{k}(c_{i_1})$, 
and $\max\{k\text{-}dist(c_j)|c_j \in N_k(c_{i_1}) \cup N_{k}(c_{i_2})\} - \min\{k\text{-}dist(c_j)|c_j \in N_k(c_{i_1}) \cup N_{k}(c_{i_2})\} \le \epsilon$.
Let $\overline{reach_k}(c_{i_1})$ and $\overline{reach_k}(c_{i_2})$ denote the average reachability distance of $c_{i_1}$ and $c_{i_2}$
% and $N_{k}(c_{i_2})\setminus{c_{i_1}}=N_{k}(c_{i_1})\setminus{c_{i_2}}$,
% from the same neighborhood.
% They 
% who are in each other's $k$-distance neighborhood and share the remaining $k$-nearest neighbors,
We have  
% their local reachability density will be quite similar, where the variation is mainly caused by the client difference in $k$-$dist$:
% For clients $c_i$ and $c$
\begin{align*}
    & lrd_k(c_{i_1}) = 1/\overline{reach_k}(c_{i_1})\\
    =\,& 1/(\frac{\sum_{c_{j}\in N_k(c_{i_1})} reach_{k}(c_{i_1}, c_j)}{|N_k(c_{i_1})|} )\\
    =\,&1/(\frac{\sum_{c_{j}\in N_k(c_{i_1})\setminus{c_{i_2}}} reach_{k}(c_{i_1}, c_j)+reach_{k}(c_{i_1}, c_{i_2})}{|N_k(c_{i_1})|} )\\
    =\,&1/(\frac{\sum_{c_{j}\in N_k(c_{i_1})\setminus{c_{i_2}}}  k\text{-}dist(c_j)+k\text{-}dist(c_{i_2})}{|N_k(c_{i_1})|} )
\end{align*}
    % &\quad (Hint: N_k(c_{i_1})\setminus{c_{i_2}} = N_k(c_{i_2})\setminus{c_{i_1}} )    \\
Similarly, we have
\begin{align*}
%\quad 
lrd_k(c_{i_2}) 
% &= 1/(\frac{\sum_{c_{j}\in N_k(c_{i_2})} reach_{k}(c_{i_2}, c_j)}{|N_k(c_{i_2})|} ) \\
% &=1/(\frac{\sum_{c_{j}\in N_k(c_{i_2})\setminus{c_{i_1}}} reach_{k}(c_{i_2}, c_j)+reach_{k}(c_{i_2}, c_{i_1})}{|N_k(c_{i_2})|} )\\
=1/(\frac{\sum_{c_{j}\in N_k(c_{i_2})\setminus{c_{i_1}}}k\text{-}dist(c_j)+k\text{-}dist(c_{i_1})}{|N_k(c_{i_2})|} )
\end{align*}
Let $N_k^{\mathsf{d}}$ and  $N_k^{\mathsf{c}}$ denote the set of $k$-nearest neighbors that differ for $c_{i_1}$ and $c_{i_2}$ and the set of common neighbors, respectively, and $\mathsf{const}$ denote the multiplication result of the average reachability distance of $c_{i_1}$ and $c_{i_2}$, i.e.,  $\mathsf{const}=\overline{reach_k}(c_{i_1})*\overline{reach_k}(c_{i_2})$.
% Without loss of generality, let 
Then we have
\begin{align*}
    & |lrd_k(c_{i_1})-lrd_k(c_{i_2})|\\
    =\,&|1/\overline{reach_k}(c_{i_1})-1/\overline{reach_k}(c_{i_2})|\\
    =\,&|\frac{\overline{reach_k}(c_{i_2})-\overline{reach_k}(c_{i_1})}{\overline{reach_k}(c_{i_1})*\overline{reach_k}(c_{i_2})}|\\
    \le\, & \frac{|\sum_{c_{j}\in N_k^{\mathsf{d}}(c_{i_1})}  k\text{-}dist(c_j)-\sum_{c_{j}\in N_k^{\mathsf{d}}(c_{i_2})}  k\text{-}dist(c_j)|}{\min
    \{|N_k(c_{i_1})|,|N_k(c_{i_2})|\}} / \mathsf{const}+ \\
    & \frac{|\sum_{c_{j}\in N_k^{\mathsf{c}}(c_{i_1})}  k\text{-}dist(c_j)-\sum_{c_{j}\in N_k^{\mathsf{c}}(c_{i_2})}  k\text{-}dist(c_j)|}{\min
    \{|N_k(c_{i_1})|,|N_k(c_{i_2})|\}} / \mathsf{const} \\
    =\,& \frac{|\sum_{c_{j}\in N_k^{\mathsf{d}}(c_{i_1})}  k\text{-}dist(c_j)-\sum_{c_{j}\in N_k^{\mathsf{d}}(c_{i_2})}  k\text{-}dist(c_j)|}{\min
    \{|N_k(c_{i_1})|,|N_k(c_{i_2})|\}} / \mathsf{const}\\
    \le\,& \frac{\epsilon}{\mathsf{const}}.
\end{align*}
    % \text{and} reach_{k}(c_{i_1},c_j)=reach_{k}(c_{i_2},c_j)=k\text{-}dist(c_j)
    % &=1/(\frac{\sum_{c_{j}\in N_k(c_{i_2})\setminus{c_{i_1}}} reach_{k}(c_{i_2}, c_j)+k\text{-}dist(c_{i_2})}{|N_k(c_{i_2})|} )\\
% \begin{align*}
%     &lrd_k(c_{i_1}) = 1/(\frac{\sum_{c_{j}\in N_k(c_{i_1})} reach_{k}(c_{i_1}, c_j)}{|N_k(c_{i_1})|} )\\
%     &=1/(\frac{\sum_{c_{j}\in N_k(c_{i_1})\setminus{c_{i_2}}} reach_{k}(c_{i_1}, c_j)+reach_{k}(c_{i_1}, c_{i_2})}{|N_k(c_{i_1})|} )\\
%     &=1/(\frac{\sum_{c_{j}\in N_k(c_{i_1})\setminus{c_{i_2}}}  k\text{-}dist(c_j)+k\text{-}dist(c_{i_2})}{|N_k(c_{i_1})|} )\\
%     % &\quad (Hint: N_k(c_{i_1})\setminus{c_{i_2}} = N_k(c_{i_2})\setminus{c_{i_1}} )    \\
%     &\approx 1/(\frac{\sum_{c_{j}\in N_k(c_{i_2})\setminus{c_{i_1}}}k\text{-}dist(c_j)+k\text{-}dist(c_{i_1})}{|N_k(c_{i_2})|} )\\
%     % \text{and} reach_{k}(c_{i_1},c_j)=reach_{k}(c_{i_2},c_j)=k\text{-}dist(c_j)
%     % &=1/(\frac{\sum_{c_{j}\in N_k(c_{i_2})\setminus{c_{i_1}}} reach_{k}(c_{i_2}, c_j)+k\text{-}dist(c_{i_2})}{|N_k(c_{i_2})|} )\\
%     &=1/(\frac{\sum_{c_{j}\in N_k(c_{i_2})\setminus{c_{i_1}}} reach_{k}(c_{i_2}, c_j)+reach_{k}(c_{i_2}, c_{i_1})}{|N_k(c_{i_2})|} )\\
%     &= lrd_k(c_{i_2})
% \end{align*}
\end{proof}}
        % &\quad (Hint: N_k(c_{i_1})\setminus{c_{i_2}} = N_k(c_{i_2})\setminus{c_{i_1}} )    \\
\lemmaMali*
\begin{proof}
For any malicious client $c_i$, 
% according to Assumption~\ref{assume3}, 
there are benign clients involved in its $k$-distance neighborhood.
We denote it as $N_{k}(c_i)=N_k^{\mathsf{B}}(c_i)\cup N_k^{\mathsf{M}}(c_i)$ where $N_k^{\mathsf{B}}(c_i)$ denotes the set of benign clients and $N_k^{\mathsf{M}}(c_i)$ denotes the set of malicious ones.
Hence, we have
\begin{align*}
   & lrd_k(c_i)\\
   =\,& 1/\frac{\sum_{c_{j}\in N_k(c_{i})} reach_{k}(c_i, c_j)}{|N_k(c_i)|} \\
    =\,&1/\frac{\sum_{c^{\mathsf{M}}_{j}\in N^{\mathsf{M}}_k(c_{i})} reach_{k}(c_i, c^{\mathsf{M}}_j)+\sum_{c^{\mathsf{B}}_{j}\in N^{\mathsf{B}}_k(c_{i})} reach_{k}(c_i, c^{\mathsf{B}}_j)}{|N_k(c_i)|} \\
    =\,&1/\frac{\sum_{c^{\mathsf{M}}_{j}\in N^{\mathsf{M}}_k(c_{i})} reach_{k}(c_i, c^{\mathsf{M}}_j)+\sum_{c^{\mathsf{B}}_{j}\in N^{\mathsf{B}}_k(c_{i})} d(c_i, c^{\mathsf{B}}_j)}{|N_k(c_i)|} 
\end{align*}
Because of the sparsity of malicious clients, the reachability distance between malicious clients is greater than the distance between benign clients, i.e., for $c_i^{\mathsf{M}}, c_j^{\mathsf{M}} \in \mathcal{M}$,
for $c_i^{\mathsf{B}},  c_j^{\mathsf{B}} \in \mathcal{B}$, we have 
$reach_k(c_i^{\mathsf{M}}, c_j^{\mathsf{M}})>reach_k(c_i^{\mathsf{B}}, c_j^{\mathsf{B}})$.
And for benign clients $c_j^{\mathsf{B}} \in N^{\mathsf{B}}_k(c_{i})$, we have $d(c_i, c_j^{\mathsf{B}})>k\text{-}dist(c_j^{\mathsf{B}})$.
\xz{Let $N^{\mathsf{B},\mathsf{c}}_k(c_{i}^{\mathsf{B}})$ and $N^{\mathsf{B},\mathsf{d}}_k(c_{i}^{\mathsf{B}})$ denote the set of common and different benign neighbors between $c_{i}^{\mathsf{B}}$ and $c_{i}$, i.e., $N^{\mathsf{B},\mathsf{c}}_k(c_{i}^{\mathsf{B}})=N^{\mathsf{B}}_k(c_{i})\cap N^{\mathsf{B}}_k(c_{i}^{\mathsf{B}})$ and $N^{\mathsf{B},\mathsf{d}}_k(c_{i}^{\mathsf{B}})=N^{\mathsf{B}}_k(c_{i}^{\mathsf{B}})\setminus{ N^{\mathsf{B}}_k(c_{i})}$.
Then for a benign client $c_i^{\mathsf{B}} \in N_k^{\mathsf{B}}(c_i)$, 
% \ning{change $c_i^{\mathsf{B}}$ to a different notation} 
it holds that}
\xz{
\begin{align*}
   & lrd_k(c_i)    \\
   =\,&1/\frac{\sum_{c^{\mathsf{M}}_{j}\in N^{\mathsf{M}}_k(c_{i})} reach_{k}(c_i, c^{\mathsf{M}}_j)+\sum_{c^{\mathsf{B}}_{j}\in N^{\mathsf{B}}_k(c_{i})} d(c_i, c^{\mathsf{B}}_j)}{|N_k(c_i)|} \\
       <\,&1/\frac{\sum_{c^{\mathsf{B}}_{j}\in N^{\mathsf{B},\mathsf{d}}_k(c_{i}^{\mathsf{B}})} reach_{k}(c_i^{\mathsf{B}}, c^{\mathsf{B}}_j)+\sum_{c^{\mathsf{B}}_{j}\in N^{\mathsf{B},\mathsf{c}}_k(c_{i}^{\mathsf{B}})} k\text{-}dist(c_j^{\mathsf{B}})}{|N_k(c_i^{\mathsf{B}})|} \\
    % &<1/\frac{\sum_{c^{\mathsf{B}}_{j}\in N^{\mathsf{B}}_k(c_{i}^{\mathsf{B}})\setminus{ N^{\mathsf{B}}_k(c_{i})}} reach_{k}(c_i^{\mathsf{B}}, c^{\mathsf{B}}_j)+\sum_{c^{\mathsf{B}}_{j}\in N^{\mathsf{B}}_k(c_{i})\cap N^{\mathsf{B}}_k(c_{i}^{\mathsf{B}})} k\text{-}dist(c_j^{\mathsf{B}})}{|N_k(c_i^{\mathsf{B}})|} \\
    =\,&lrd_{k}(c_i^{\mathsf{B}})
\end{align*}
}
\end{proof}

\lofBenign*
\begin{proof}
For all $k$-nearest neighbors $c_j$ of $c$, it holds that $reach_k(c, c_j)\le \mathsf{reach}_{max}$. 
Hence,
\begin{align*}
   lrd(c)&= 1/(\frac{\sum_{c_j\in N_k(c)} reach_{k}(c, c_j)}{|N_k(c)|} )\\ 
   &\ge 1/(\frac{\sum_{c_j\in N_k(c)} \mathsf{reach}_{max}}{|N_k(c)|} )\\
   &= 1/\mathsf{reach}_{max}
\end{align*}
Similarly, it holds that $\forall c_j \in N_{k}(c)$, $reach_k(c, c_j)\ge \mathsf{reach}_{min}$.
Hence, we have $lrd(c) \le 1/\mathsf{reach}_{min}$.
Same property also holds for $k$-nearest neighbors of $c$, i.e., $\forall c_j \in N_{k}(c)$, $1/\mathsf{reach}_{max} \le lrd(c_j) \le 1/\mathsf{reach}_{min}$.
Therefore, 
\begin{align*}
    LOF_k(c) &= \frac{1}{|N_k(c)|} \sum_{c_j\in N_{k}(c)} \frac{lrd_k(c_j)}{lrd_k(c)}\\
    &\le \frac{1}{|N_k(c)|} \sum_{c_j\in N_{k}(c)} \frac{1/\mathsf{reach}_{min}}{1/\mathsf{reach}_{max}}\\
    &=\frac{\mathsf{reach}_{max}}{\mathsf{reach}_{min}}=1+\epsilon
\end{align*}
Similarly, it holds that
$LOF_k(c) \ge \frac{\mathsf{reach}_{min}}{\mathsf{reach}_{max}}=\frac{1}{1+\epsilon}$
\end{proof}

\lofGeneral*
\begin{proof}
$\forall c' \in N_k(c)$, $reach_k(c,c')\ge \mathsf{reach}^{c}_{min}$.
Then according to Definition 3, 
\begin{equation*}
    lrd_k(c)\le \frac{1}{\mathsf{reach}^{c}_{min}}
\end{equation*}
$\forall c_j \in N_k(c')$, $reach_k(c', c_j) \le \mathsf{reach}^{N}_{max}$.
Then we have
\begin{equation*}
    lrd_k(c')\ge \frac{1}{\mathsf{reach}^{N}_{max}}
\end{equation*}
Hence, it holds that
\begin{align*}
    LOF_k(c)&= \frac{1}{|N_k(c)|} \sum_{c'\in N_{k}(c)} \frac{lrd_k(c')}{lrd_k(c)}\\
    &\ge \frac{1}{|N_k(c)|} \sum_{c'\in N_{k}(c)}\frac{1/\mathsf{reach}^{N}_{max}}{1/\mathsf{reach}^{c}_{min}}\\
    &=  \frac{\mathsf{reach}^{c}_{min}}{\mathsf{reach}^{N}_{max}}
\end{align*}
Similarly, it holds that
\begin{equation*}
LOF_k(c) \le \frac{\mathsf{reach}^{c}_{max}}{\mathsf{reach}^{N}_{min}}
\end{equation*}
\end{proof}

\lbLOF*
\begin{proof}
Assume a remaining malicious client $c_j$,
according to Theorem \ref{theorem:general-lof},
the LOF lower bound depends on the ratio of minimum reachability distance of the malicious client against the maximum one of its neighbors, 
% i.e., 
$\mathcal{LB}(LOF^{t}(c_j))=\frac{\mathsf{reach}^{c_j}_{min}}{\mathsf{reach}^{N}_{max}}$. 
    We denote its original minimum reachability distance with $\mathsf{reach}_{min}$, maximum reachability distance of its neighbors $\mathsf{reach}^{N}_{max}$, and updated ones after one iteration with $\mathsf{reach}'_{min}$, $\mathsf{reach}'^{N}_{max}$. 
    The following properties hold:
    \begin{enumerate}
    
        \item  $\mathsf{reach}'_{min} \ge \mathsf{reach}_{min}$. If $\mathsf{reach}_{min}$ is attained between $c_j$ and a removed  malicious client. Then we have $\mathsf{reach}'_{min} > \mathsf{reach}_{min}$. Otherwise, $\mathsf{reach}_{min}$ stays the same.
        \item   $\mathsf{reach}'^{N}_{max} \le \mathsf{reach}^{N}_{max}$.
    If $\mathsf{reach}^{N}_{max}$ is attained by a removed malicious client, with benign neighbors substituting the malicious ones, we have $\mathsf{reach}'^{N}_{max} < \mathsf{reach}^{N}_{max}$.
    Otherwise, it stays the same.
    Due to the density of benign clients, $\mathsf{reach}^{N}_{max}$ is generally attained by the malicious neighbors with larger deviation.
    With the elimination of such neighbors, the updated neighbors will have smaller $\mathsf{reach}'^{N}_{max}$.
    \end{enumerate}
    Based on properties (1) and (2),
    we have 
    \begin{equation*}
        \mathcal{LB}(LOF^{t}(c_j))=\frac{\mathsf{reach}_{min}}{\mathsf{reach}^{N}_{max}} \le \frac{\mathsf{reach}'_{min}}{\mathsf{reach}'^{N}_{max}} = \mathcal{LB}(LOF^{t+1}(c_j))
    \end{equation*}
\end{proof}

% use appendices with more than one appendix
% then use \section to start each appendix
% you must declare a \section before using any
% \subsection or using \label (\appendices by itself
% starts a section numbered zero.)
%

% \appendices
% \section{Proof of the First Zonklar Equation}
% Appendix one text goes here.

% % you can choose not to have a title for an appendix
% % if you want by leaving the argument blank
% \section{}
% Appendix two text goes here.
